# Supplementary material for: Lossless Acceleration of Large Language Model via Adaptive N-gram Parallel Decoding
Source: arXiv:2404.08698 source file (2024-07-10)
Supplement: Supplementary file 1 [file appendix.tex]

\appendix

\section{Appendix}
\subsection{Standard Autoregressive Decoding}
\label{app:autoregression}

Transformer-based LLMs use autoregressive decoding, taking text input ($x_1, ..., x_{t-1}$) to predict the next token probability, $p(x_{t}|x_1, ..., x_{t-1})$. Efficiency is improved by caching past states as $p(x_{t}|(k,v)_1, ..., (k,v)_{t-1})$. This is an autoregressive process, LLM can only predict one token at a time, as subsequent tokens are dependent on the previous token.%Users choose between greedy decoding (picking the most probable token for deterministic output), and sampling (introduces variability). Both methods suit various needs. However, memory bandwidth constraints still limit decoding efficiency. Caching reduces parameter access per token, but bandwidth impacts speed and inference time.

\subsection{Parallel Decoding Analysis}
\label{app:exp_Parallel_inference_speed}
\begin{figure}[h!]
    \centering
    \includegraphics[width=0.45\textwidth]{imgs/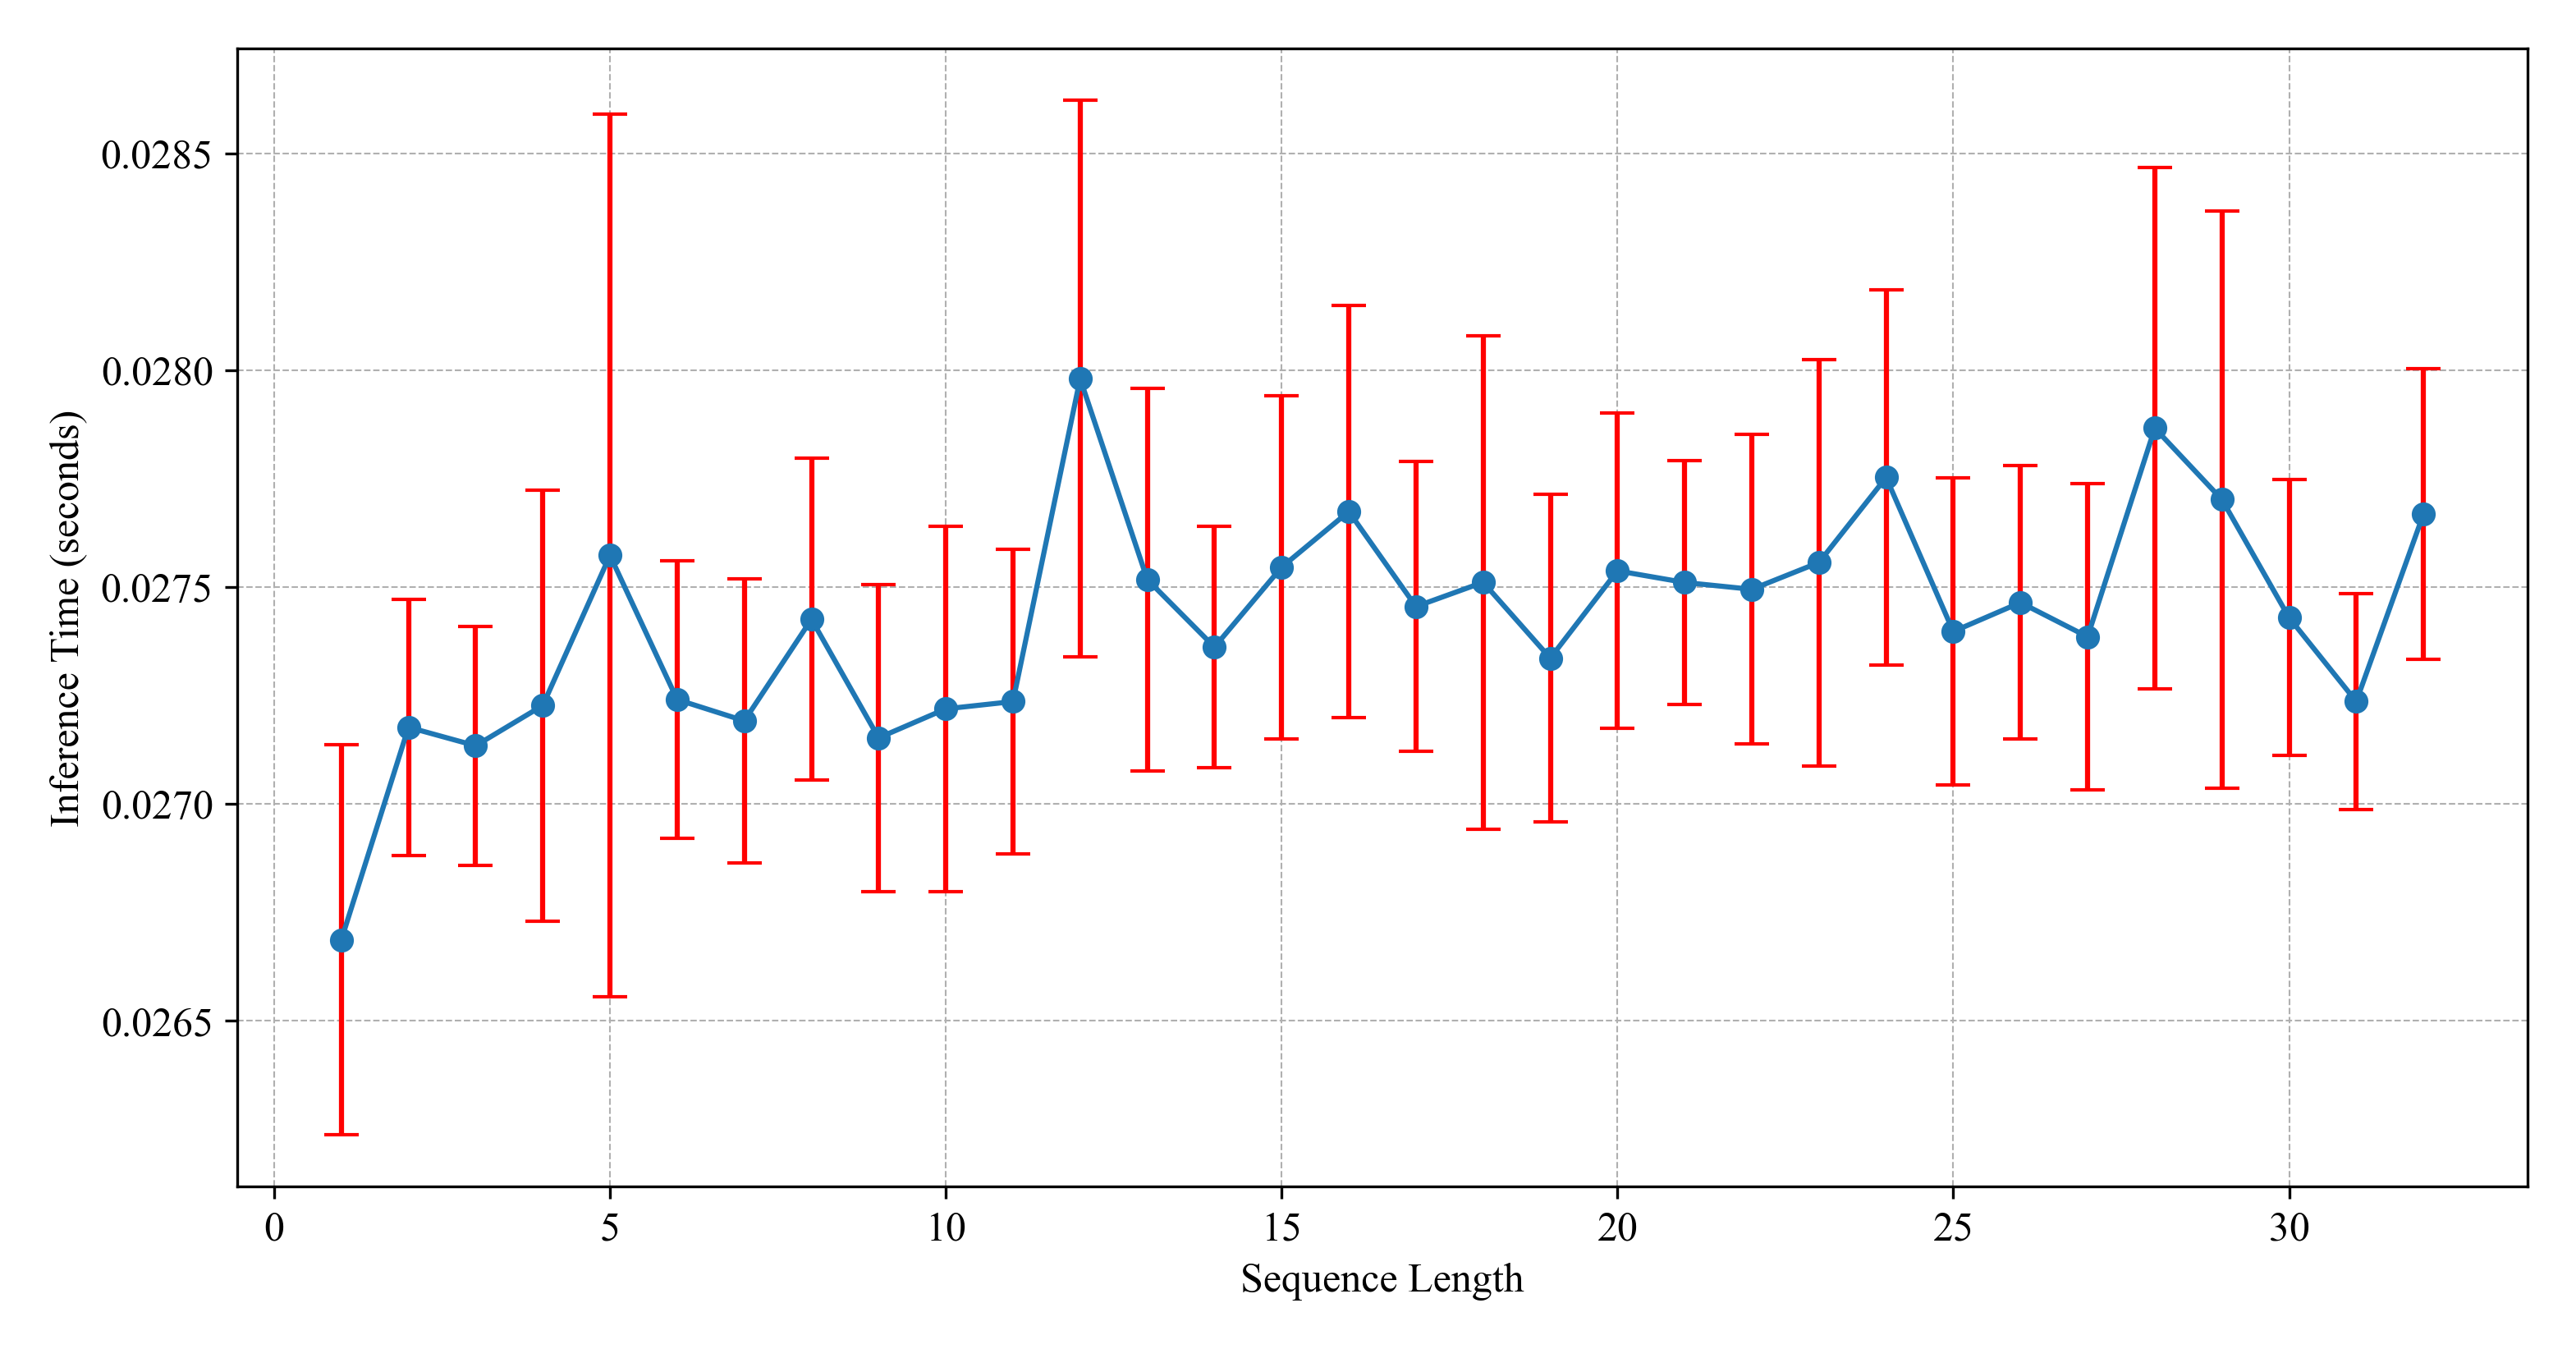}
    \caption{A single decoding step latency of LLaMA-7B is recorded with different $K$.}
    \label{fig:2}
\end{figure}
Figure \ref{fig:2} evaluates the latency impact of processing varying numbers of tokens in the parallel decoding step while maintaining a constant prompt size of 512 tokens in the key-value (KV) cache. The results indicate that small increments in $K$ do not significantly affect latency. It provides the opportunity to verify multiple draft tokens simultaneously without incurring significant additional latency.

\subsection{Algorithm Details}
\label{app:alg1_details}
In Algorithm 1, the complete process of our ANPD is demonstrated. The variable $K$ denotes the length of the draft output (draft steps), $M$ signifies the maximum length for LLM generation, and $O$ is an output list utilized for recording the token ids of the generated tokens. The presented algorithm initiates by utilizing a prompt to generate token ids, which are then stored in the N-gram module Memory. As delineated in line 6 of the pseudocode, the LLM engages in the prefill phase to produce a valid token prediction (\textit{pred}). This token is essential for updating the output $O$, the Memory, and the draft array $drafts$.
% The decoding loop, spanning lines 8 to the last, commences by slicing the most recent $N-1$ tokens from the complete token ids, serving as the Query's input. During the draft generation phase, the draft's tokens are continually employed to refresh this Query input. Subsequently, parallel decoding is executed on the drafts at line 17, then each token within the draft is meticulously compared with the LLM's predictions for consistency.
The decoding initiates with the slicing of the most recent $N-1$ tokens from the complete token ids ($token\_ids$), these tokens are then utilized as the input for the $QUERY$ in the decoding loop, which spans from line 8 to the terminal line of the algorithm. Throughout the draft generation phase, the tokens within the draft are dynamically updated by  $QUERY$. Subsequently, at line 17, parallel decoding is applied to the drafts. This is followed by a meticulous comparison of each token in the draft against the predictions rendered by the large language model (LLM) to ensure alignment and consistency.
% The comparison ceases when a discrepancy arises at the $j^{th}$ draft. At this juncture, the draft reverts to the preceding token offered by the LLM to initiate the subsequent drafting. if all the draft's content is verified, the last LLM predict token will be used for new drafting.
The comparison process is halted upon the detection of a divergence at the $j^{th}$ draft token. At this critical point, the procedure reverts to the next token of the last consistent token provided by the large language model (LLM) to commence a new draft iteration. If the entire content of the draft withstands verification, the final token predicted by the LLM is then adopted to initiate the generation of a new draft sequence.

\subsection{Alpaca Train Details}
\label{app:finetune}
% The methodology adopted for training the model, Alpaca-7B, is in accordance with the guidelines delineated by \citep{alpaca}, utilizing the dataset they introduced, comprising approximately 52,000 training instances. For the purpose of fine-tuning the LLaMA-7b model, the learning rate was set to \(2 \times 10^{-5}\), with a batch size of 128, and epochs is 3. To facilitate effective training within the computational constraints, the gradient\_accumulation\_steps parameter was used, we used float16 for training, engaging the stage2 optimization of DeepSpeed and enabling gradient\_checkpointing on one NVIDIA-A100 GPU.
We train the Alpaca-7B model followed by \citep{alpaca}. The training dataset employed consists of approximately 52,000 instances, as introduced in \citep{alpaca}. 
For fine-tuning the LLaMA-7b model, the learning rate was set to \(2 \times 10^{-5}\), with a batch size of 128, across a total of 3 epochs. To facilitate effective training within the computational constraints, the $gradient\_accumulation\_steps$ parameter was used. We used float16 for training, engaging the $stage2$ optimization of DeepSpeed and enabling $gradient\_checkpointing$ on one NVIDIA-A100 GPU.

In the case of Alpaca-CNN/DM-7B, we random sample a subset of 30,000 data samples from the CNN/DM trainset, following the alpaca template provided by \citep{alpaca}, as shown in Figure \ref{fig:alpaca template}. Notably, the remaining training hyperparameters are the same as Alpaca-7B, except the number of epochs is 5.

\begin{figure}[ht]
\centering
\begin{Verbatim}[breaklines=true, commandchars=\\\{\}]
Below is an instruction that describes a task, paired with an input that provides further context. Write a response that appropriately completes the request.

### Instruction:
\{instruction\}

### Input:
\{input\}

### Response:
\end{Verbatim}
\caption{Alpaca template, the instruction is "Summarize the following articles." in our experiments.}
\label{fig:alpaca template}
\end{figure}

\subsection{Evaluation}
\label{app:eval}
% Our ANPD does not modify the model's output. Tables~\ref{tab:metric cnndm} and~\ref{tab:metric humaneval} present the testing outcomes for various models on the standard CNN/DM and HumanEval datasets, respectively. It should be noted that the results exhibit some inconsistencies, which can be attributed to a recognized issue\footnote{https://github.com/huggingface/transformers/issues/25420}, however, the overall impact is deemed to be minimal.
% We employed a 1-shot evaluation for non-instruction tuned models with ROUGE-2 scores for summarization and 0-shot with pass@1 metrics for code generation, metric result are in Appendix~\ref{app:eval}, our approach presented herein does not alter the output or computational processes of existing Large Language Models (LLMs), thus maintaining their fundamental performance, there will be no comparative analysis on accuracy.
% Our evaluation involved a 1-shot setup for non-instruction tuned models using ROUGE-2 scores to assess text summarization and a 0-shot setup with pass@1 metrics for code generation. The results of these metrics can be found in Appendix~\ref{app:eval}. It is important to note that our approach does not modify the fundamental output or computational processes of existing Large Language Models (LLMs), thereby preserving their inherent performance capabilities. As a result, a comparative analysis regarding accuracy has not been included.
Our evaluation involved a 1-shot setup for non-instruction tuned models and a 0-shot setting for instruction-tuned models, both using ROUGE-2 scores to assess text summarization. For code generation, a 0-shot setting with pass@1 metrics was employed. It is important to note that our approach does not modify the fundamental output or computational processes of existing Large Language Models (LLMs), thereby preserving their inherent performance capabilities. %Consequently, a comparative analysis regarding accuracy has not been included.
Therefore, we do not conduct a detailed analysis of the accuracy in this paper. For the 0-shot setting, the alpaca template illustrated in Figure~\ref{fig:alpaca template} is utilized for the summarization task. For the 1-shot setting, the input template employed is depicted in Figure~\ref{fig:1-shot template}. Regarding the use of CodeLLaMA for HuamnEval, we directly enter the text corresponding to the prompt keyword of the sample content, and corresponding instructions have been written for each sample.

\begin{figure}[ht]
\centering
\begin{Verbatim}[breaklines=true, commandchars=\\\{\}]
Article: \{shot_article\}
Summary: \{shot_summary\}
Article: \{article\}
Summary: 
\end{Verbatim}
\caption{1-shot Template.}
\label{fig:1-shot template}
\end{figure}

Our proposed ANPD maintains the integrity of the original model's predictive performance. As delineated in Tables~\ref{tab:metric_cnndm} and~\ref{tab:metric_humaneval}, we report the empirical evaluation results on the widely-adopted benchmarks CNN/DM and HumanEval, respectively. Notwithstanding minor discrepancies in the findings, these can be ascribed to a documented caching anomaly in the issue\footnote{https://github.com/huggingface/transformers/issues/25420}; nonetheless, their influence on the overall efficacy of ANPD is negligible.

\begin{table}[h]
    \centering
    \scalebox{0.75}{
    \begin{tabular}{|c|c|c|c|}
    \hline
       Method  & shot & ANPD & CNN/DM  \\
       \hline
        LLaMA-7B & 1 &  & 8.66  \\
        LLaMA-7B  & 1 & \checkmark & 8.64  \\
        Alpaca-7B  & 0 & & 10.84  \\
        
        Alpaca-7B & 0& \checkmark &10.83 \\
        Alpaca-CNN/DM-7B & 0& &17.16\\
         Alpaca-CNN/DM-7B & 0&\checkmark &17.23\\
    \hline
    \hline
      LLaMA-2-13B & 1 &  & 10.58  \\
        LLaMA-2-13B  & 1 & \checkmark & 10.61  \\

        \hline
        \hline
    
    ChatGLM3-6B & 0 &  & 14.60 \\
    ChatGLM3-6B & 0 & \checkmark & 14.54 \\
    \hline
    \end{tabular}
    }
    \caption{The comparison of the ROUGE-2 for CNN/DM.}
    \label{tab:metric_cnndm}
\end{table}

\begin{table}[h]
    \centering
    \scalebox{0.75}{
    \begin{tabular}{|c|c|c|c|}
    \hline
       Method  & shot & ANPD & HumanEval  \\
       \hline
        CodeLLaMA-7B & 0 &  & 0.3109  \\
        CodeLLaMA-7B  & 0 & \checkmark &  0.3109 \\
        CodeLLaMA-13B & 0 &  & 0.3415  \\
        CodeLLaMA-13B  & 0 & \checkmark & 0.3415  \\
    \hline
    \end{tabular}
    }
    \caption{The comparison of the  Pass@1 for HumanEval.}
    \label{tab:metric_humaneval}
\end{table}
% , HumanEval we use Pass @1.

% \begin{table}[ht]
%     \centering
%     \scalebox{0.65}{
%     \begin{tabular}{|c|c|c|c|c|c|}
%     \hline
%        Method  & shot & ANPD & CNN/DM & XSum & HumanEval\\
%        \hline
%         LLaMA-7B & 1 &  & 8.66 & 3.43 & -\\
%         LLaMA-7B  & 1 & \checkmark & 8.64 & 3.44 & - \\
%         Alpaca-7B  & 0 & & 10.84 &4.02 & -\\
        
%         Alpaca-7B & 0& \checkmark &10.83 &4.04&-\\
%         Alpaca-CNN/DM-7B & 0& &17.16&4.28&-\\
%          Alpaca-CNN/DM-7B & 0&\checkmark &17.23&4.30&-\\
%     \hline
%     \end{tabular}
%     }
%     \caption{Verification of Method Output. For summary task we use ROUGE-2, HumanEval we use Pass @1.}
%     \label{tab:metric}
% \end{table}

% \subsubsection{CNN/DM evaluation Details}

% \subsubsection{XSum Evaluation Details}

% \subsubsection{HumanEval Evaluation Details}

\subsection{Multi-Level N-gram}
\label{app:ml-gram}
\begin{figure}[h!]
    \centering
    \includegraphics[width=0.45\textwidth]{imgs/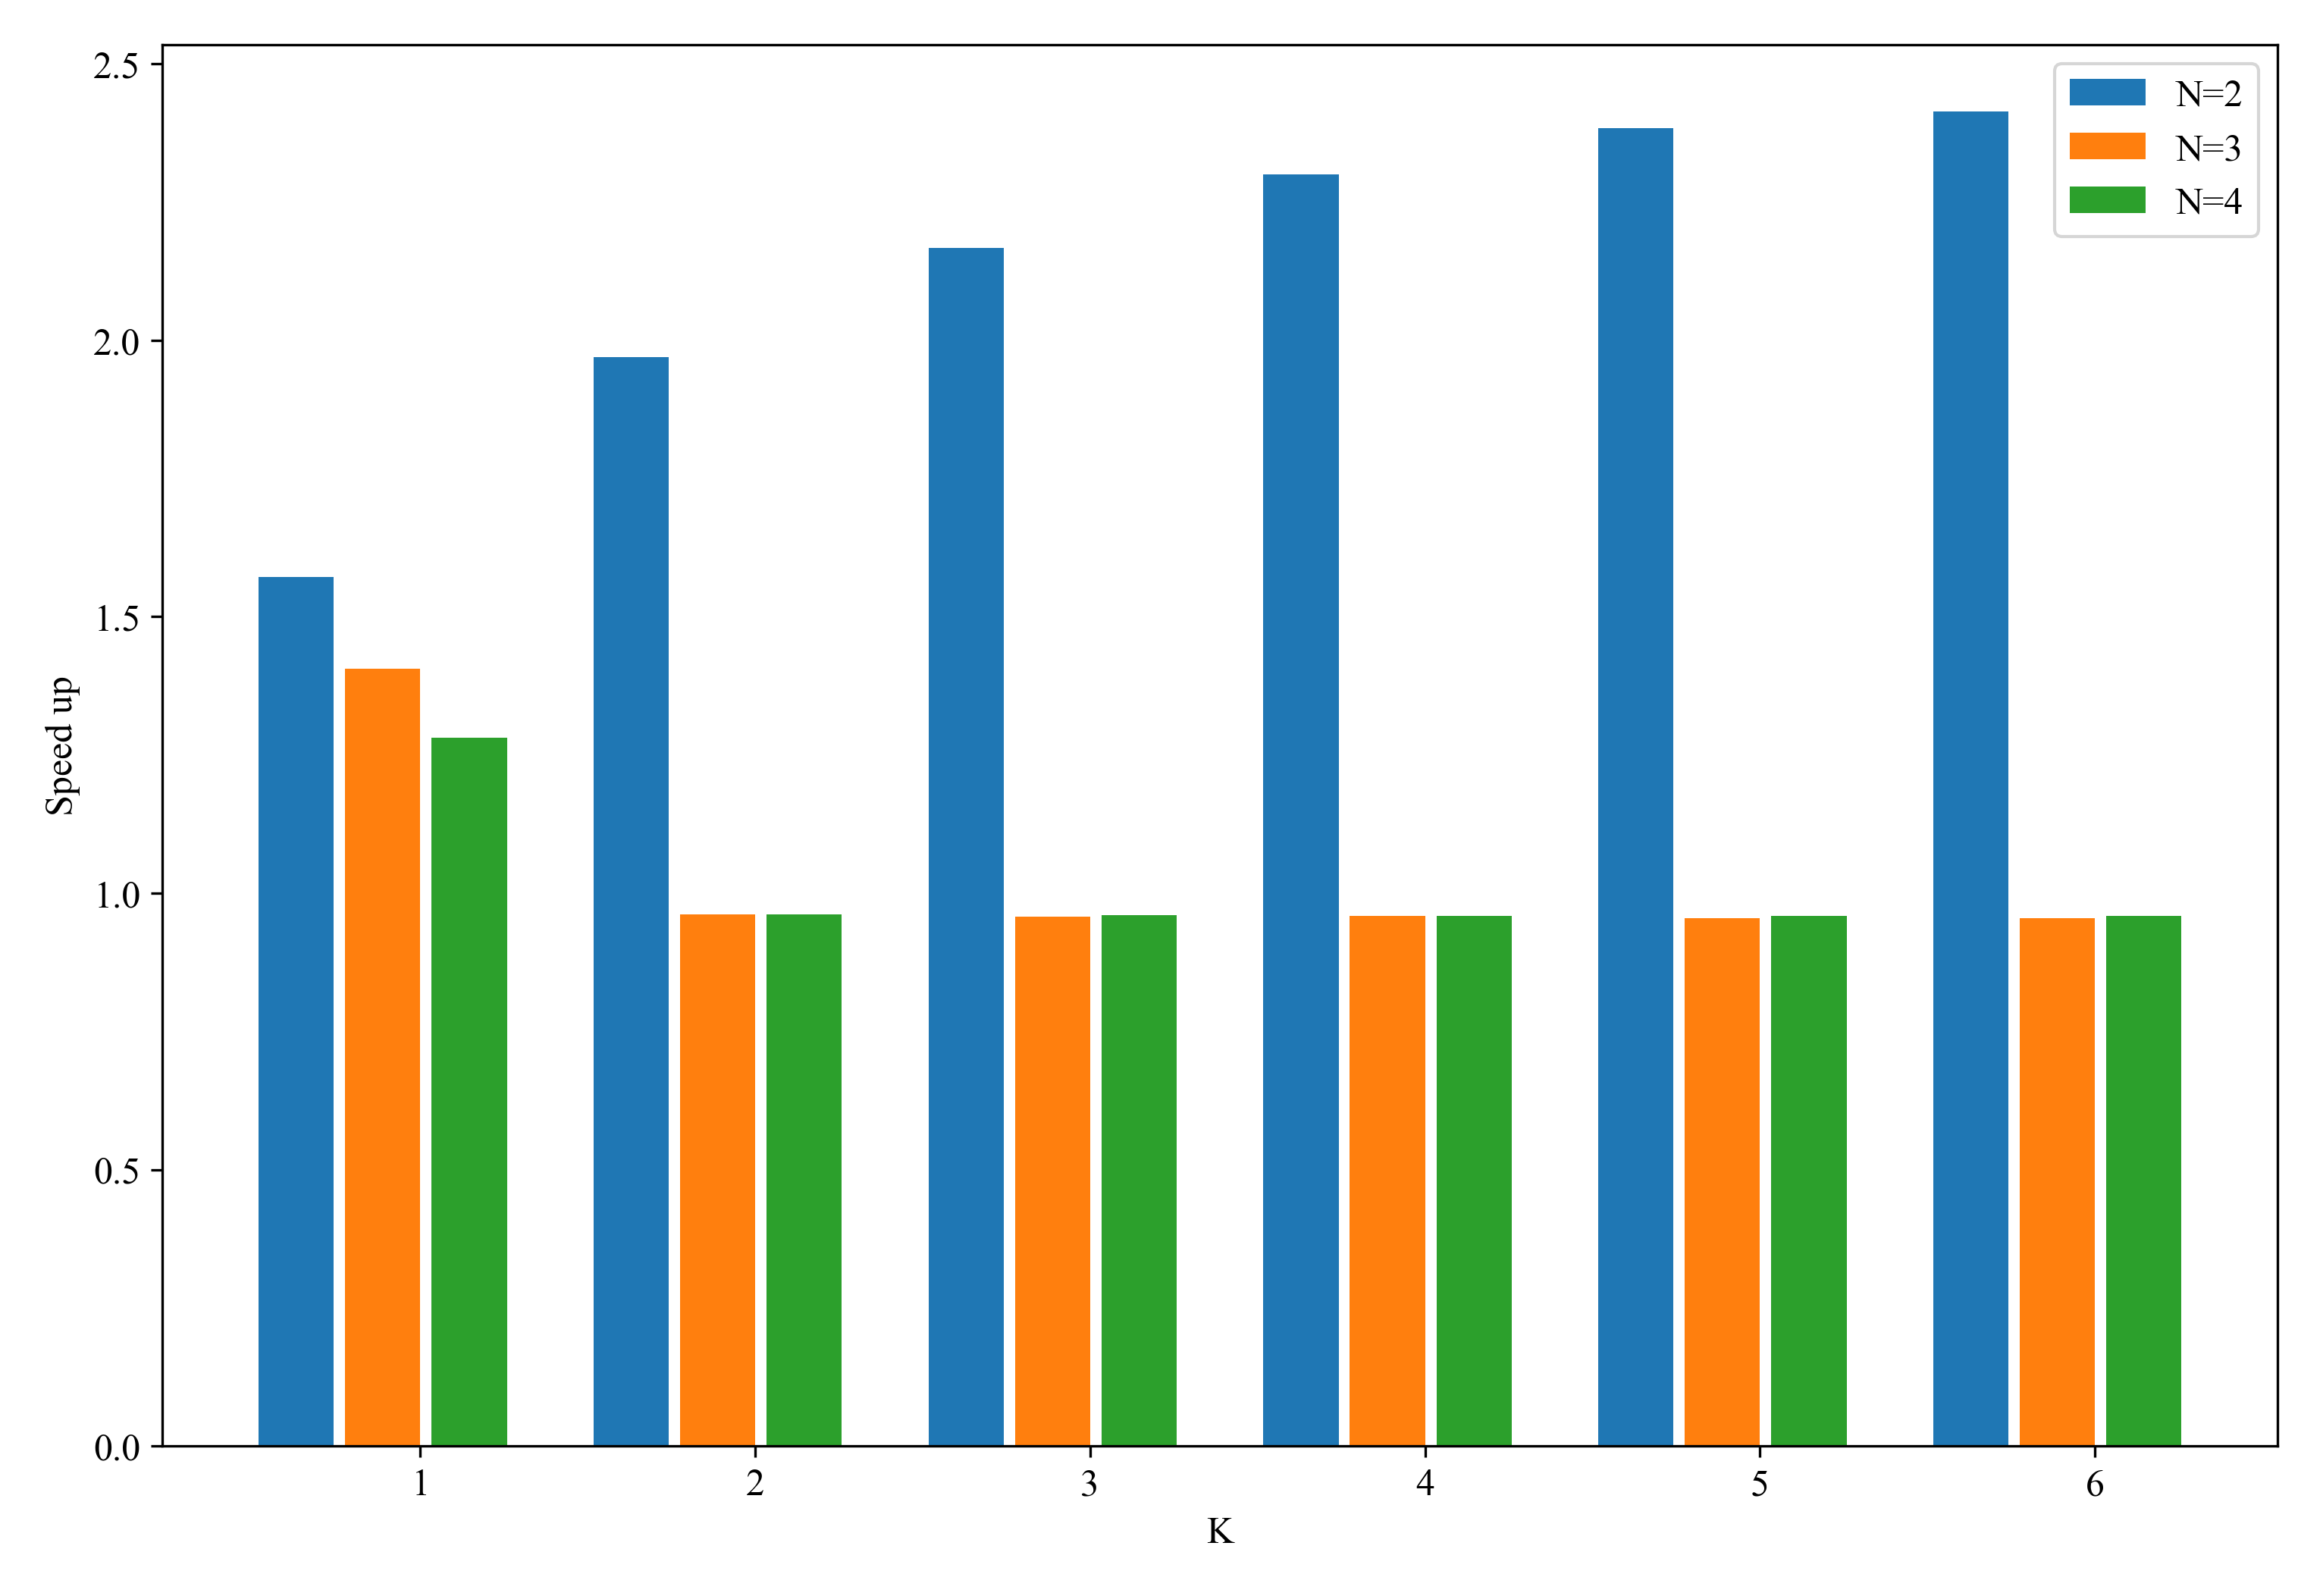}
    \caption{The acceleration comparison of the ANPD for different \( K \) and \( N \), without MLN, using the CodeLLaMA-7B.}
    \label{fig:speed_N_K_exp}
\end{figure}
% A series of controlled experiments were orchestrated to evaluate the speed enhancement of our newly proposed algorithm across different configurations determined by varying \( K \) and \( N \) values. These evaluations were grounded in the standard N-gram model, seamlessly integrated from the CodeLLaMA-7B framework. The selection process within these trials was governed by a greedy algorithmic approach, with the outcomes presented in Figure \ref{fig:speed_N_K_exp}. A counterintuitive phenomenon was observed: an increase in \( N \), theoretically expected to refine prediction accuracy, paradoxically led to a proliferation of instances with no viable matches, thereby decelerating inferential computation. Distinctively, our proposed method circumvents the Draft Model's requirement, effectively eliminating the burden of added computational costs.
In the experiment shown in Figure~\ref{fig:speed_N_K_exp}, where the Multi-Level N-gram (MLN) strategy was not utilized, we reverted to testing the original N-gram module. The results from this setting indicate that merely increasing the \( N \) value—referring to the length of the word sequences considered by the model—does not lead to a faster inference process in LLMs. This is primarily attributed to the fact that a larger \( N \) value results in fewer successful matches during the Query phase. As the N-gram sequences become longer, the likelihood of finding an exact match in the database diminishes, which in turn negates the potential gains in inference speed from expanding the N-gram size.

\begin{figure}[h!]
    \centering
    \includegraphics[width=0.45\textwidth]{imgs/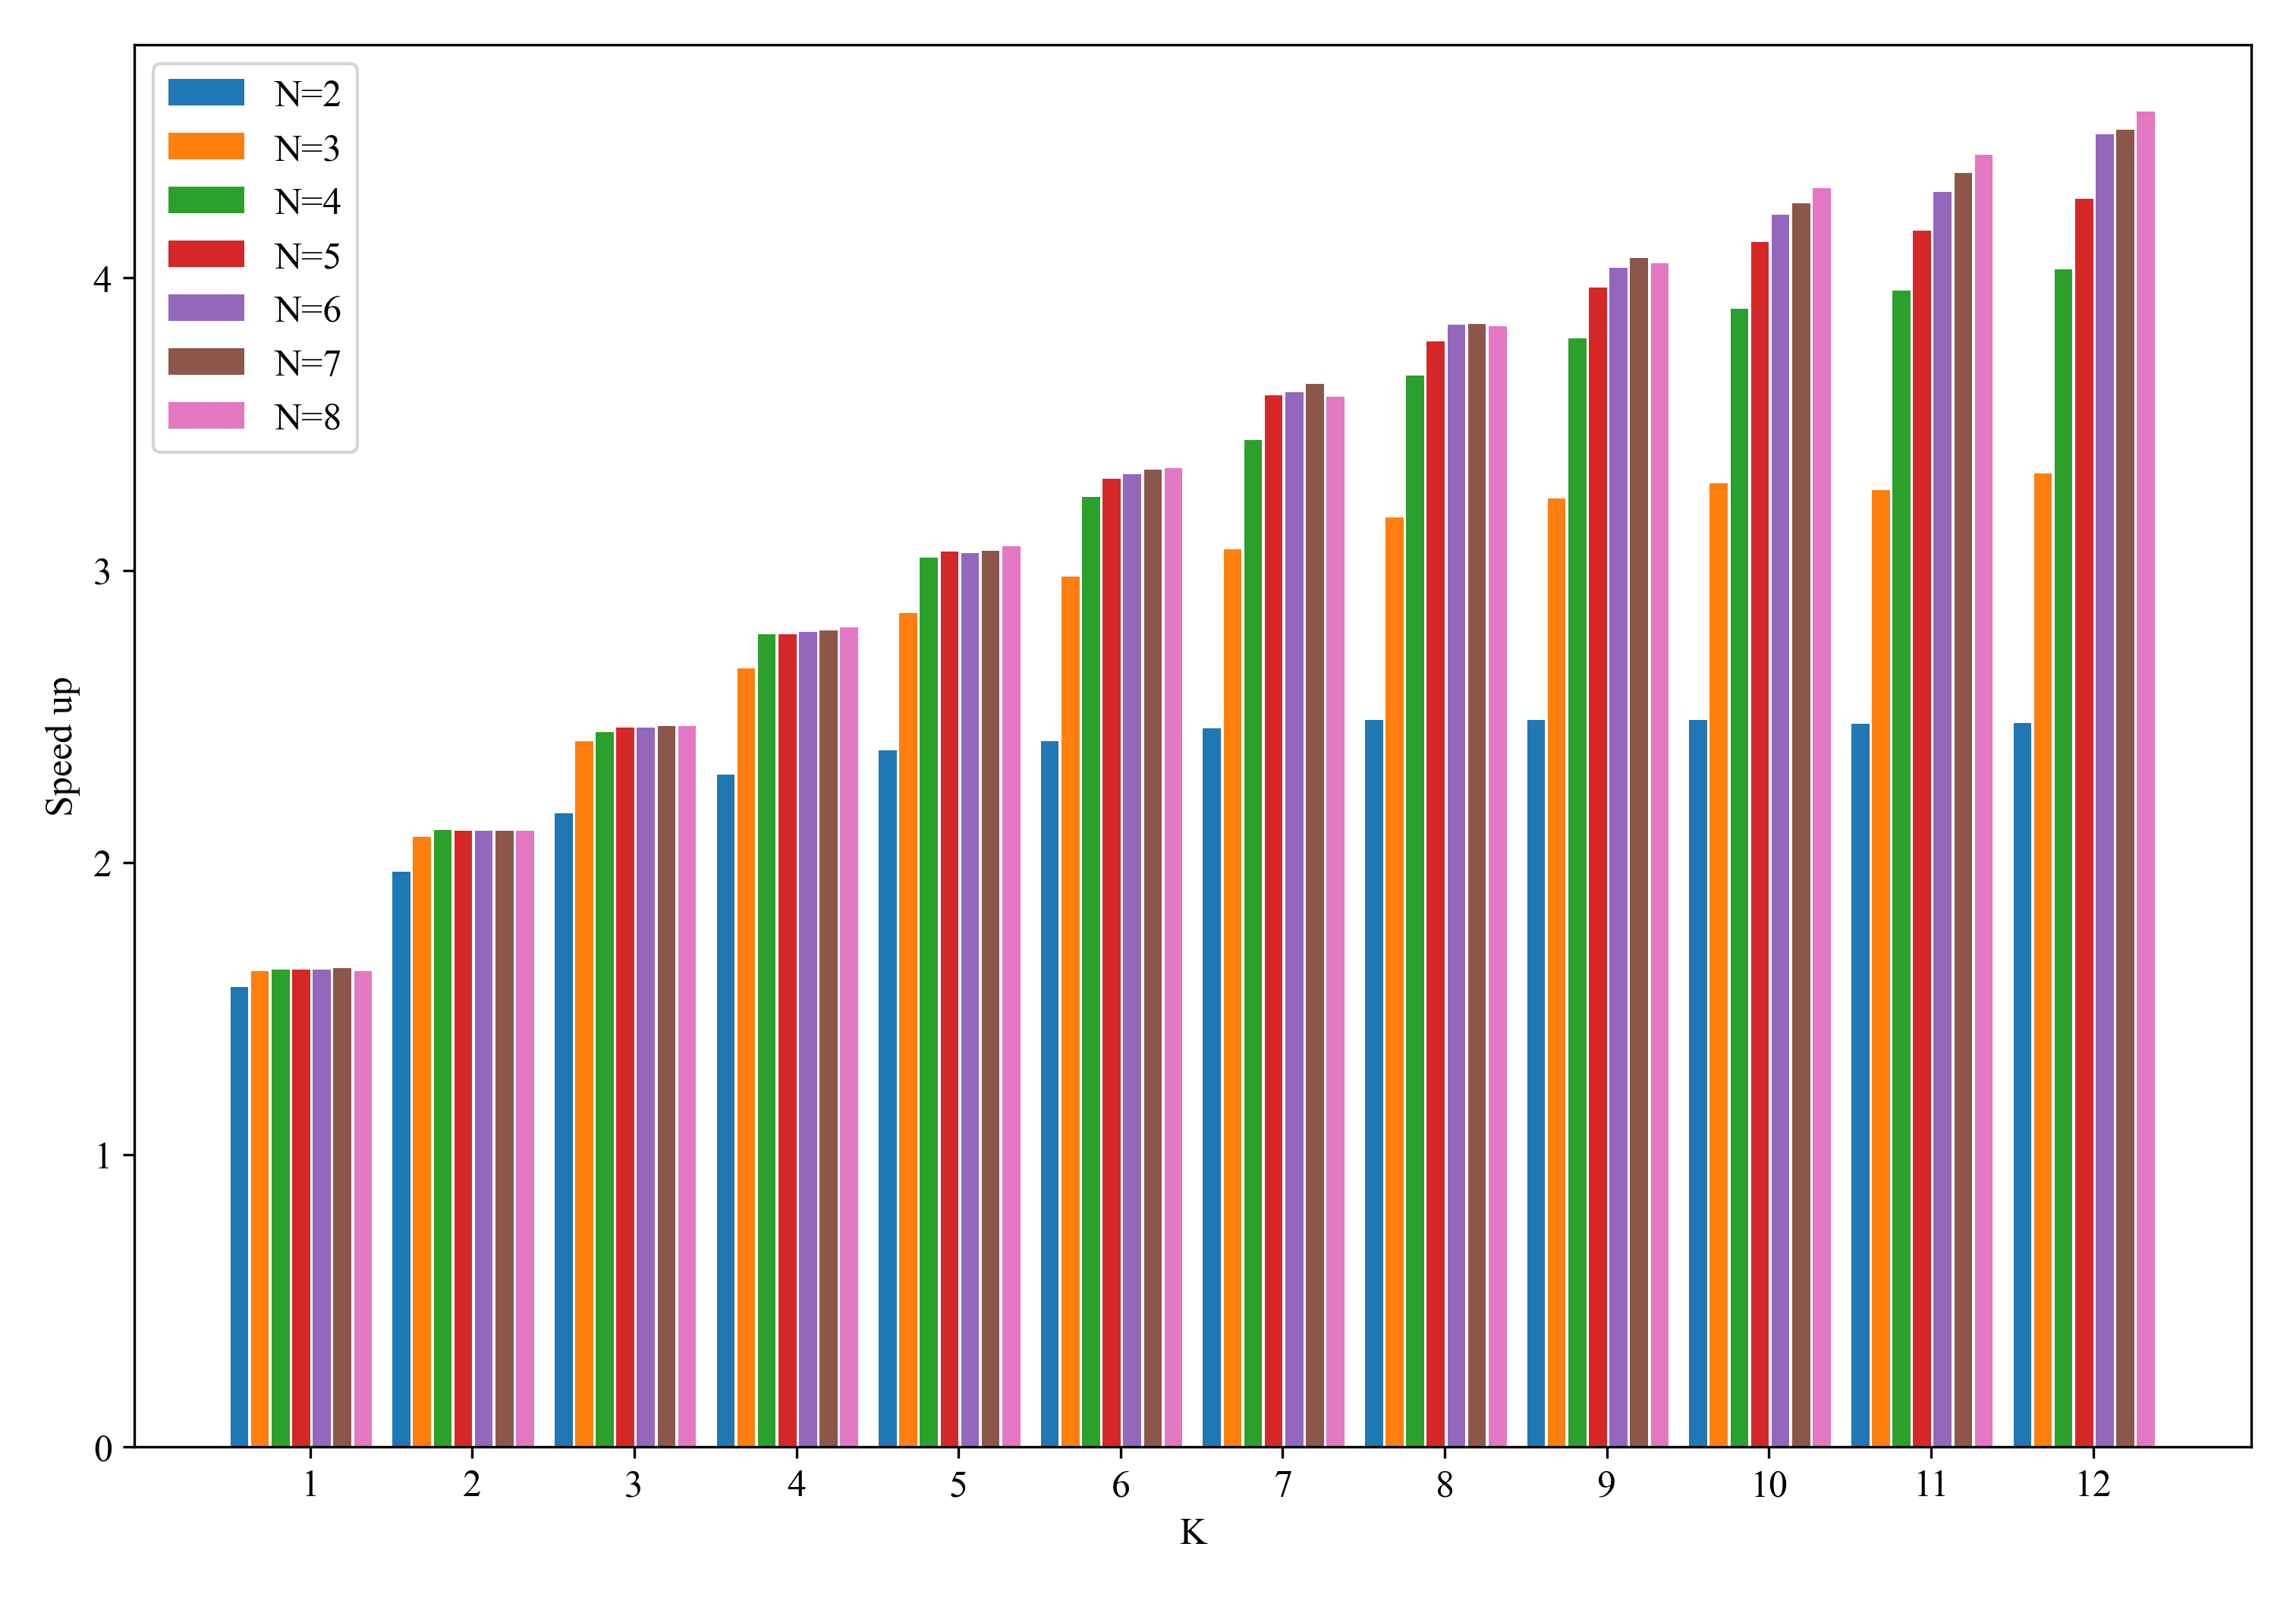}
    \caption{The acceleration comparison of the ANPD for different \( K \) and \( N \), with MLN, using the CodeLLaMA-7B.}
    \label{fig:speed_ML_N_K_exp}
\end{figure}
% As depicted in Figure.\ref{fig:speed_ML_N_K_exp}, the augmentation of the reasoning efficacy utilizing the multi-tiered N-gram approach suggested in this study is evident. Empirical analyses indicate that an optimal configuration, wherein $N$ equals 5 and $K$ is assigned a value of 7, culminates in a substantially beneficial outcome. This parameter tuning results in a reasoning acceleration factor of approximately 3.6 times the baseline speed.
Figure~\ref{fig:speed_ML_N_K_exp} Experiments on hyperparameters K and N using the CodeLLaMA model on HumanEval. Empirical analyses suggest that the setting, in which the N-gram length ($N$) is set to 5 and the number of top candidates ($K$) is set to 7, leads to a marked improvement in performance. This specific configuration yields an inference acceleration close to 3.6 $\times$ faster than the baseline. Furthermore, with a smaller N, as K increases, the acceleration effect tends to reach convergence more quickly.

\subsection{More Models}
We also conducted relevant experiments on the original OPT model~\citep{zhang2022opt} and instruction-tuned Alpaca-OPT-6.7B download from the huggingface\footnote{https://huggingface.co/Manuel030/alpaca-opt-6.7b}. The experimental results in Table~\ref{tab:opt} further verify that the ANPD we proposed has good robustness and can effectively accelerate inference for different models.
\begin{table}[h]
    \centering
    
    \begin{tabular}{|c|c|c|c|}
    \hline
    Model  & shot& CNN/DM & XSum \\ 
    \hline
    \hline
    % LLaMA-7b &  Autoregressive & 1 & - & 1 &1 & - \\
    OPT-6.7B & 1  & 3.0948x & 3.3672x  \\
    % LLaMA-13B & 1  & - & & - \\
    Alpaca-OPT-6.7B  & 0  & 3.0249x & 3.1442x  \\
    \hline

    \end{tabular}
    \caption{The comparison of acceleration effects on OPT models, $N=5$ and $K=7$.}
    \label{tab:opt}
\end{table}

\subsection{Runtime Update}
In Figure~\ref{fig:speed_up_runtime_update}, we present an experimental comparison to assess the impact of synchronizing updates to the N-gram module (denoted as Runtime Update) during the decoding stage. The comparison involved three distinct models based on LLaMA-7B, evaluated on the CNN/DM dataset. The experimental results reveal that employing a runtime update strategy enhances the acceleration of the inference process. This finding indicates that during inference, the content generated by LLMs can exhibit correlations that provide valuable guidance for the generation of content in subsequent contexts, underscoring the importance of dynamic updates within the decoding process.
\begin{figure}[h!]
    \centering
    \includegraphics[width=0.45\textwidth]{imgs/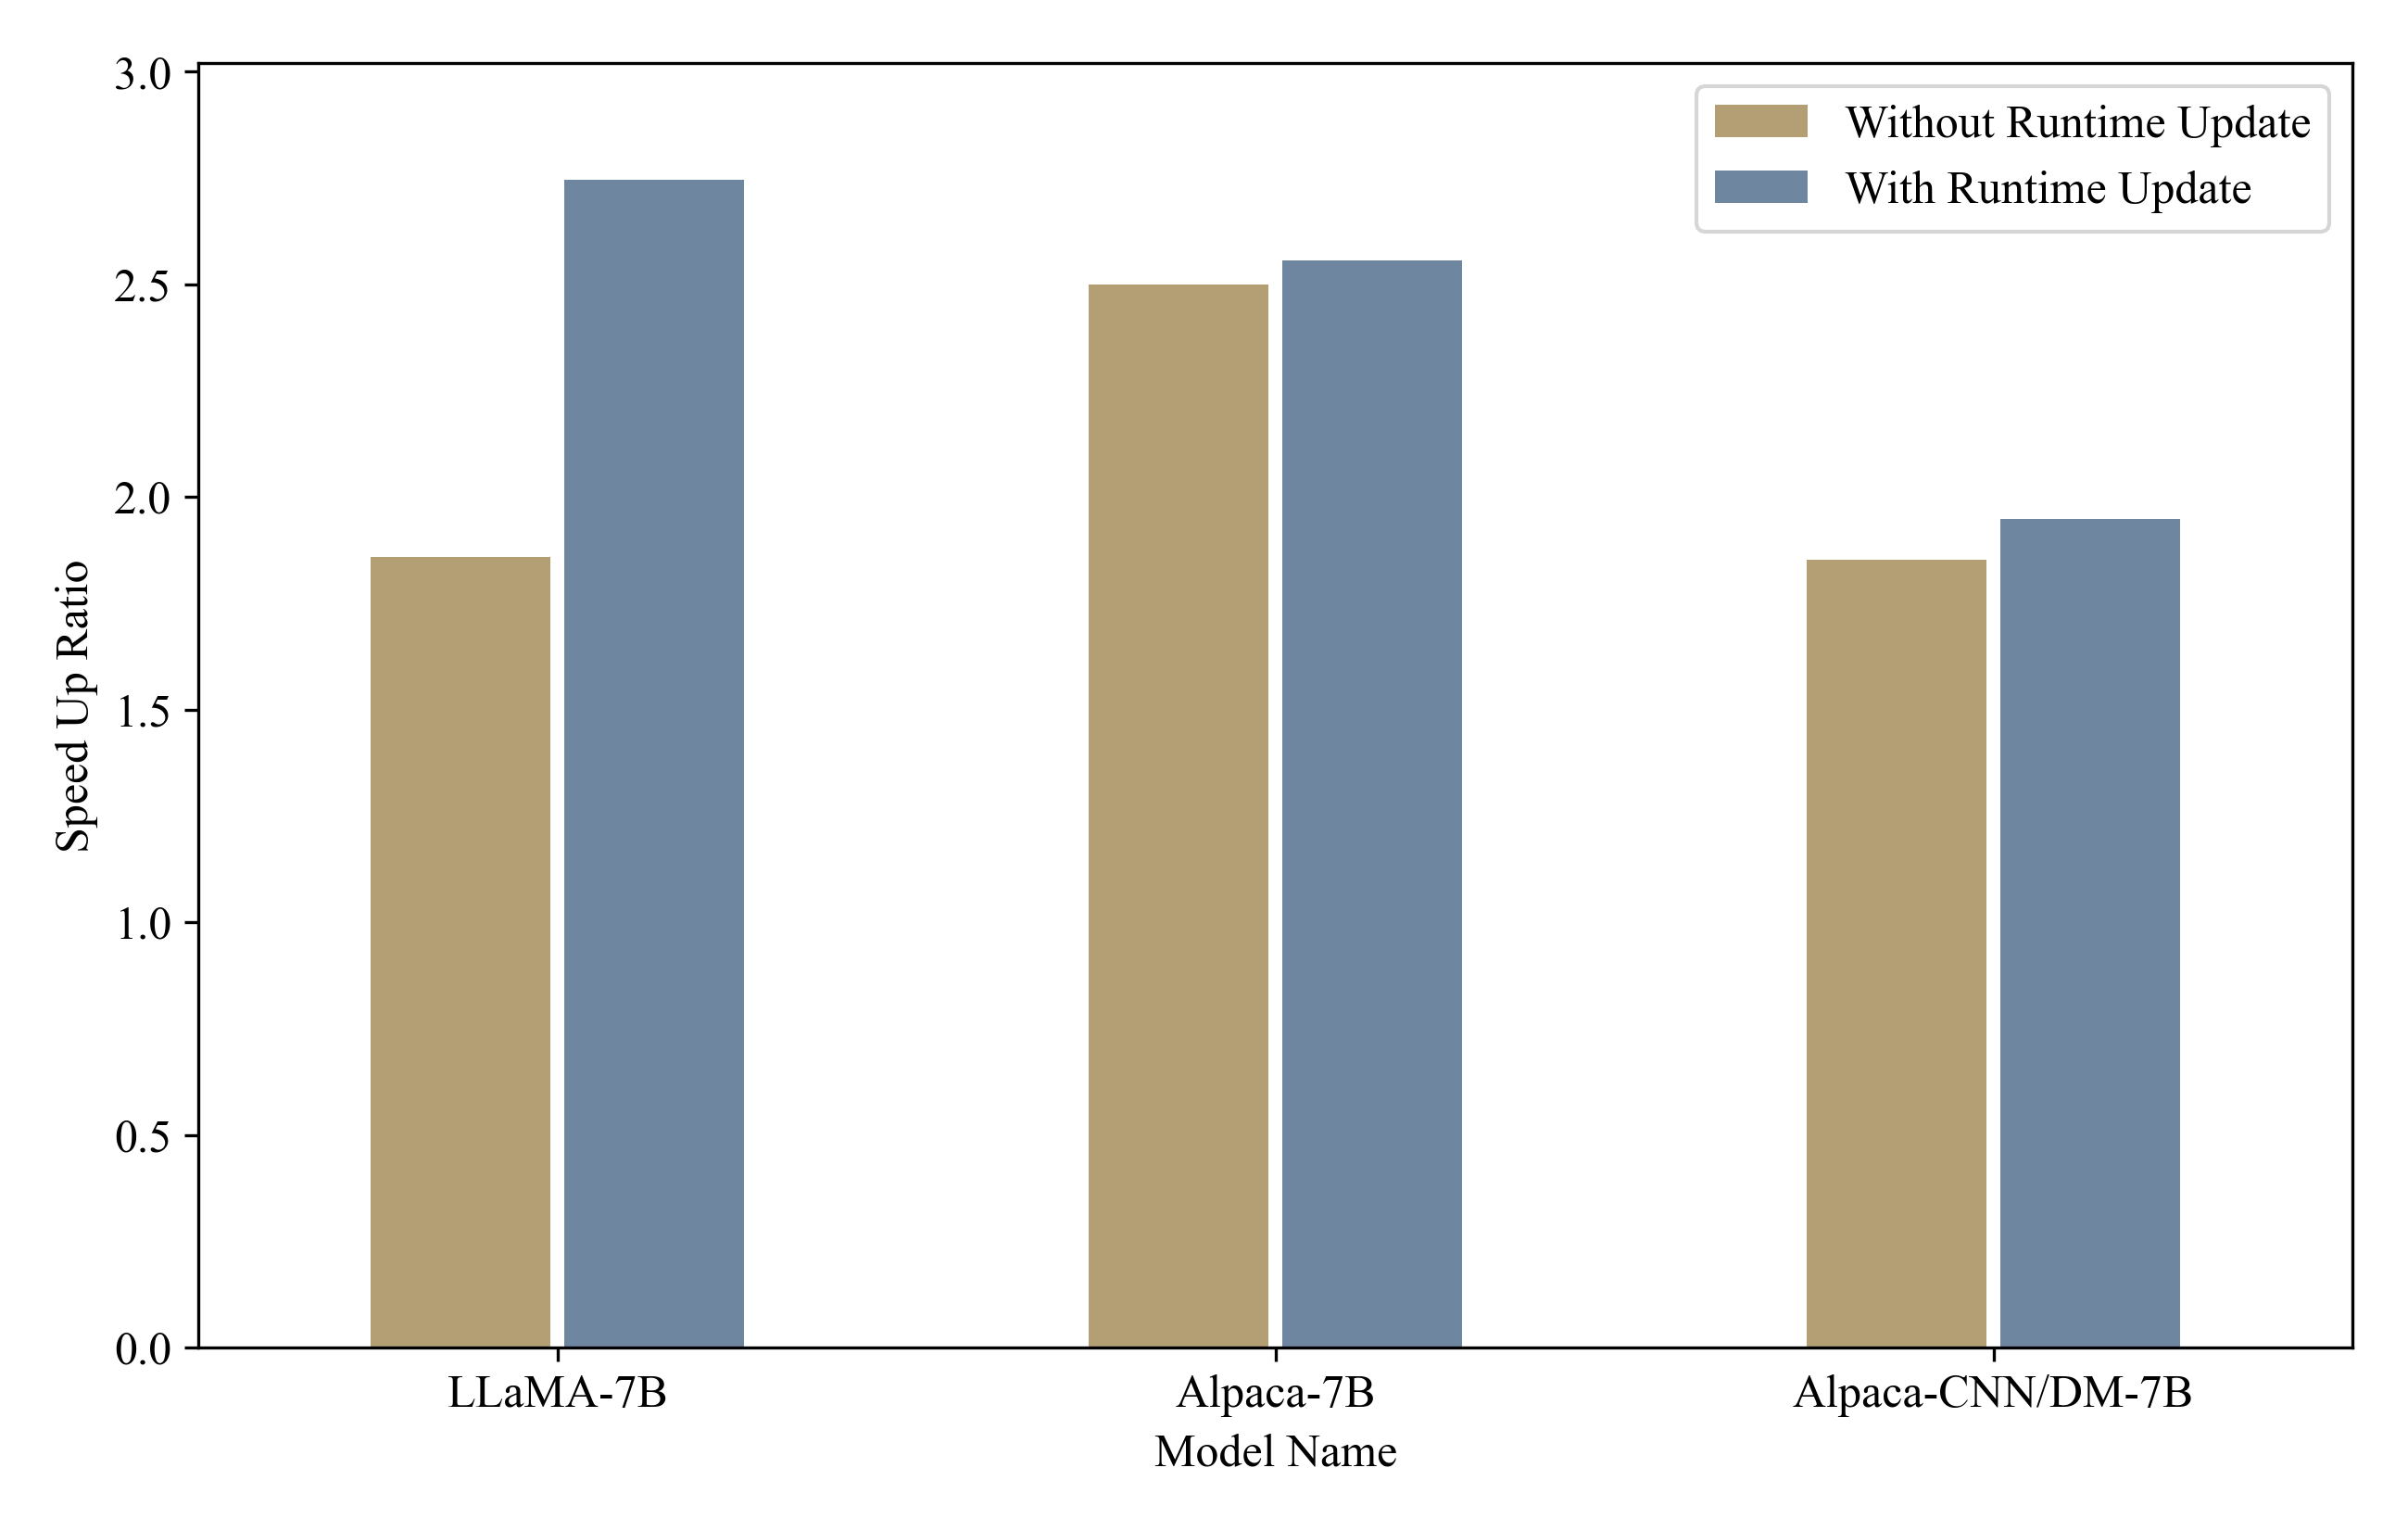}
    \caption{The comparison of acceleration effects for updating the N-gram module during decoding.}
    \label{fig:speed_up_runtime_update}
\end{figure}

\subsection{Details for Table~\ref{tab:t1}}
In Table~\ref{tab:t1}, our ANPD method utilizes a standardized configuration with $N=5$ and $K=7$. For ~\citep{zhang2023draft}, we have selected $K=12$, based on the specifications detailed in both the published paper and the open-source code. Additionally, for \citep{zhang2023draft} the draft model of the LLaMA-2-13b and CodeLLaMA-13B is constructed according to the parameters provided in the open source content\footnote{https://github.com/dilab-zju/
self-speculative-decoding}.

% \section{Appendix A}
% \label{sec:appendix2}

% This is an appendix.
